# Supplementary material for: Ranking Papers by their Short-Term Scientific Impact
Source: arXiv:2006.00951 source file (2021-04-20)
Supplement: Supplementary file 1 [file appendix.tex]

\newpage
\appendix
\section{Addendum To Evaluation}
\label{sec:appendix}

\subsection{Ranking Effectiveness}

Figure~\ref{heatmaps-full} presents heatmaps of \method's achieved correlation w.r.t. the
ground truth STI ranking, on 
the APS and hep-th datasets using the default test ratio (see
Section~\ref{sec-exp}). We observe that in all cases,
as $\beta$ approaches $0$ the correlations achieved drop
dramatically (notice the darker hues on the bottom left 
corner of each figure), while the best correlation is 
always achieved for $\beta \neq 0$, illustrating the 
importance of the newly introduced
attention-based vector.

\begin{figure*}[!ht]
\centering

\iffalse 

\begin{subfigure}{\textwidth}
  \includegraphics[width=\textwidth]{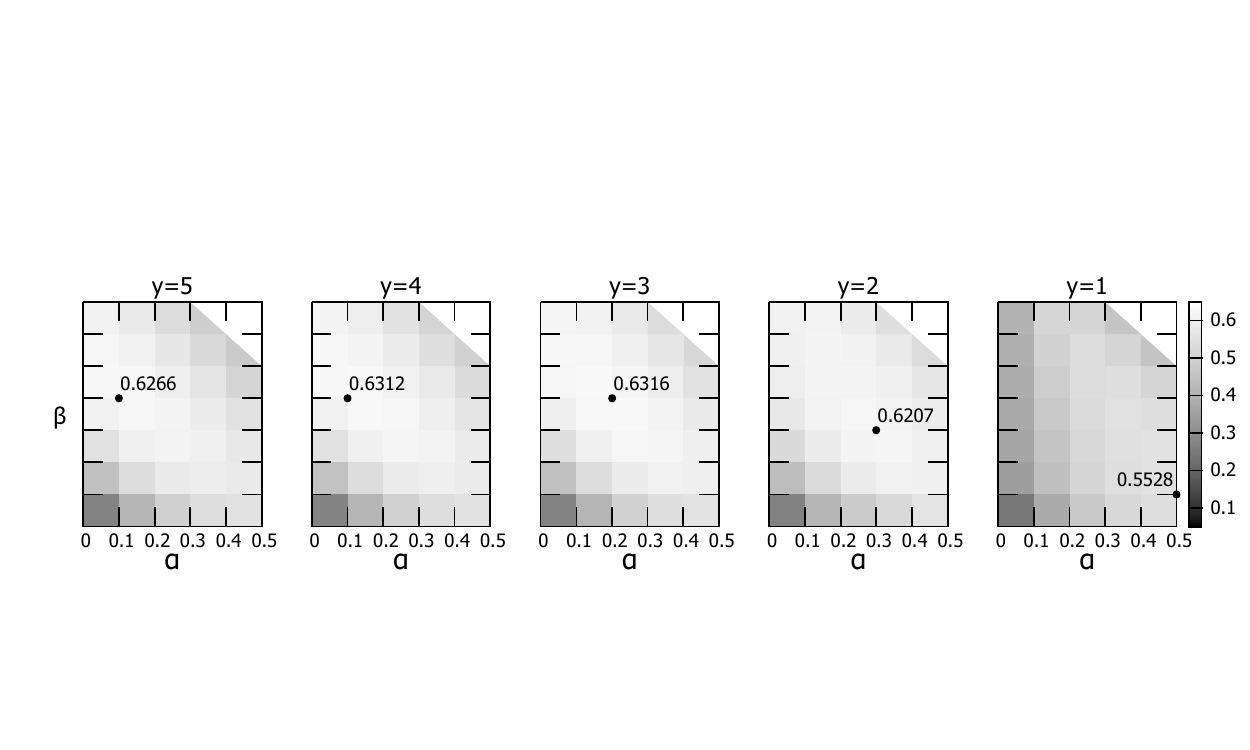}
  \caption{Correlation on the DBLP dataset.
  }
  \label{dblp_correlation_heatmap_appendix}
\end{subfigure}

\begin{subfigure}{\textwidth}
  \includegraphics[width=\textwidth]{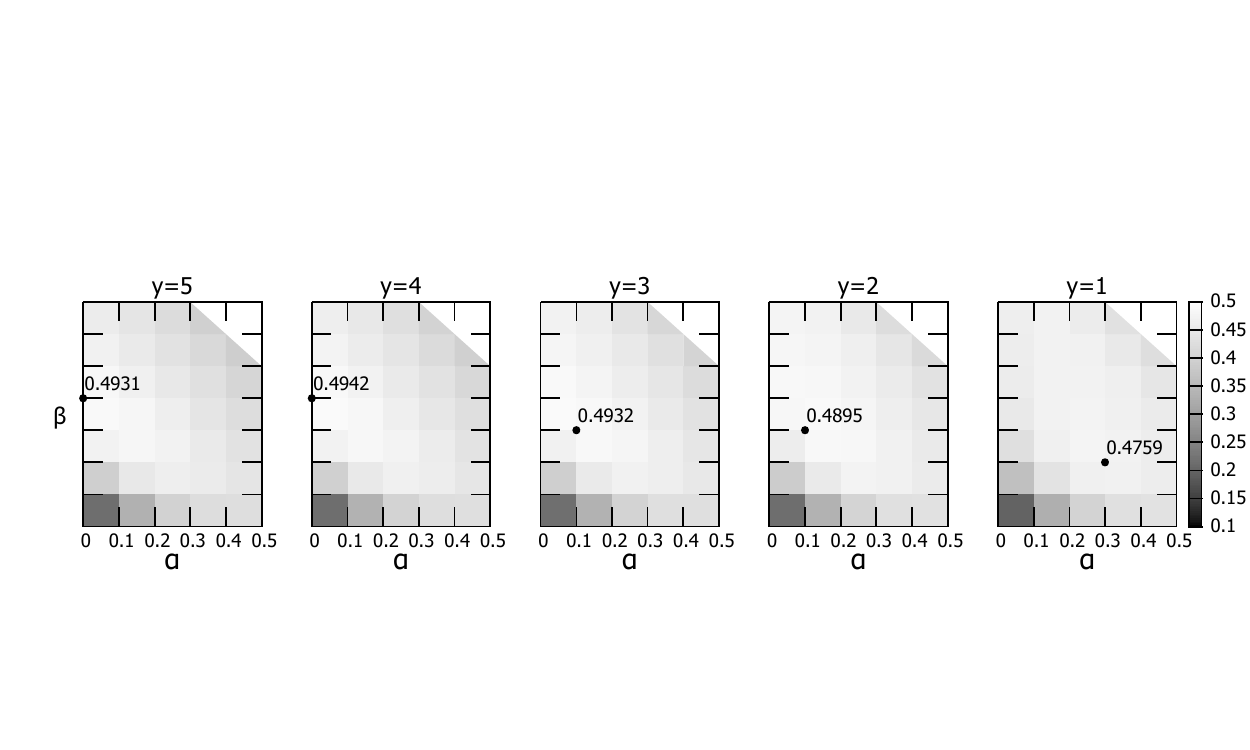}
  \caption{Correlation on the PMC dataset.
  }
  \label{pmc_correlation_heatmap_appendix}
\end{subfigure}

\fi 

\begin{subfigure}{\textwidth}
  \includegraphics[width=\textwidth]{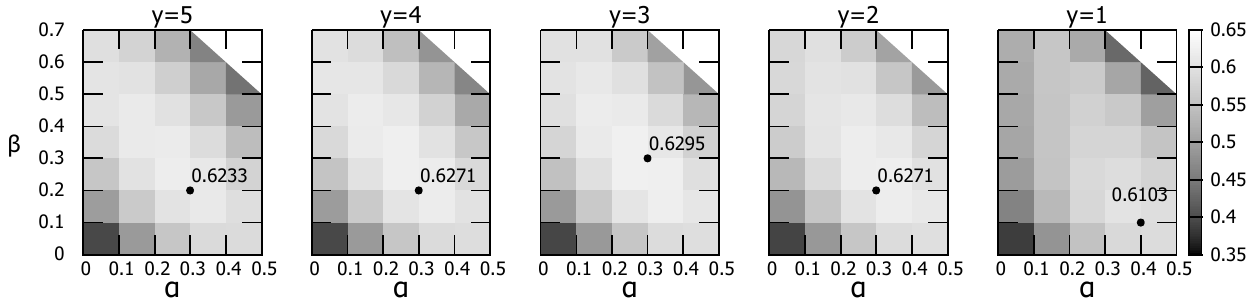}
  \caption{Correlation on the APS dataset.
  }
  \label{aps_correlation_heatmap}
\end{subfigure}

\begin{subfigure}{\textwidth}
  \includegraphics[width=\textwidth]{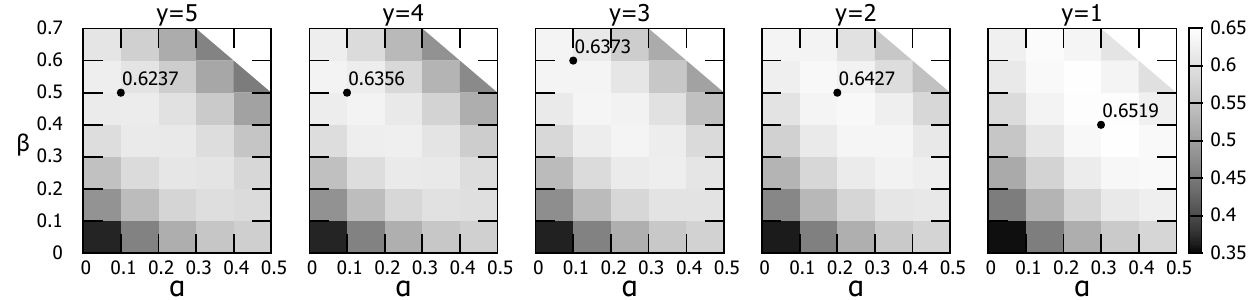}
  \caption{Correlation on the hep-th dataset.}
  \label{hepth_correlation_heatmap}
\end{subfigure}
\caption{Heatmaps depicting the effect of the parameterization of \method to its effectiveness in terms of the correlation for the APS and hep-th datasets. The best value achieved for each metric is also depicted.}
\label{heatmaps-full}

\end{figure*}

Figure~\ref{heatmaps_ndcg_full} presents heatmaps of \method's achieved nDCG@$50$ w.r.t. the
ground truth STI ranking, on 
the APS and hep-th datasets using the default test ratio.
The observations are as in the case of correlation: nCDG drops as $\beta$ approaches $0$, or as $\alpha$ increases towards
$0.5$, and its best value is achieved for some $\beta \neq 0$.

\begin{figure*}[!ht]
\centering

\iffalse 
\begin{subfigure}{\textwidth}
  \includegraphics[width=\textwidth]{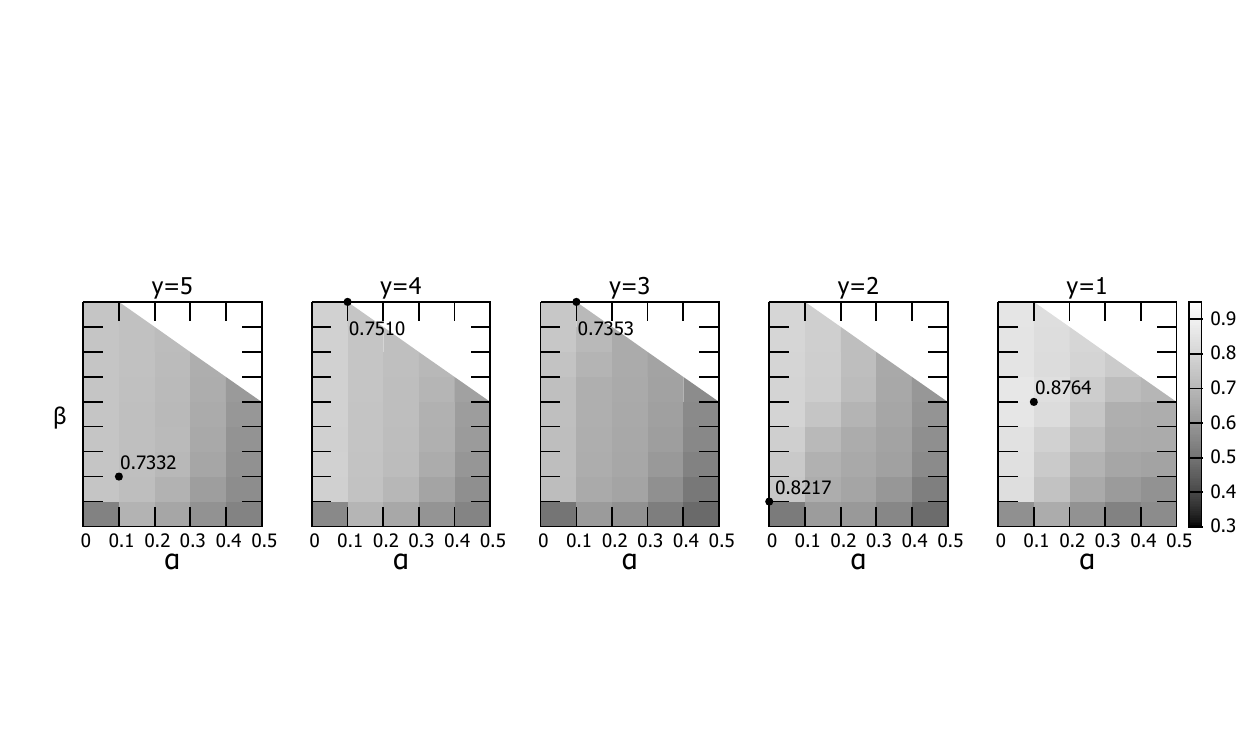}
  \caption{nDCG@50 on the DBLP dataset.}
  \label{dblp_ndcg_heatmap_appendix}
\end{subfigure}

\begin{subfigure}{\textwidth}
  \includegraphics[width=\textwidth]{figures/pmc_ndcg@50heatmap_plots_tuning_start_at0_cropped.pdf}
  \caption{nDCG@50 on the PMC dataset.
  }
  \label{pmc_ndcg_heatmap_appendix}
\end{subfigure}
\fi 

\begin{subfigure}{\textwidth}
  \includegraphics[width=\textwidth]{figures/aps_ndcg@50_plots_tuning_start_at0_cropped.pdf}
  \caption{nDCG@50 on the APS dataset.}
  \label{aps_ndcg_heatmap}
\end{subfigure}

\begin{subfigure}{\textwidth}
  \includegraphics[width=\textwidth]{figures/hepth_ndcg@50_heatmap_plots_start_at0_cropped.pdf}
  \caption{nDCG@50 on the hep-th dataset.}
  \label{hepth_ndcg_heatmap}
\end{subfigure}
\caption{Heatmaps depicting the effect of the parameterization of \method to its effectiveness in terms of nDCG@50 for the
APS and hep-th datasets. The best value achieved for each metric is also depicted.}
\label{heatmaps_ndcg_full}
\end{figure*}
